# Supplementary material for: OmniManip: Towards General Robotic Manipulation via Object-Centric Interaction Primitives as Spatial Constraints
Source: arXiv:2501.03841 source file (2025-01-07)
Supplement: Supplementary file 1 [file appendix.tex]

\clearpage
\appendix 

%%%%%%%%%%%%%%%%%%%%%%%%%%%%%%%%%%%%%%%%%%%%%%%%%%%%%%%%%%%%%%%%%%%%%%%%%%%%%%%
\section{Appendix}
\subsection{Hardware Configuration}
\label{sec:supp_hardware}
We detail our hardware setup in~\Fref{fig:supp_hardware}, which centers on a Franka Emika Panda robotic arm, a 7-DOF manipulator known for its precision and torque-controlled movements. The standard parallel gripper is equipped with UMI fingers \cite{umi}, which are flexible and can conform to objects of varying shapes, providing a more adaptable and secure grasp.
Two Intel RealSense D415 RGB-D cameras are utilized for perception. One camera is mounted on the gripper, providing a first-person view from the robot's perspective, while the other is positioned opposite the robot to offer a third-person view of the workspace. This setup facilitates both detailed object perception and overall scene understanding.
The system is powered by a workstation equipped with an Intel Core i7 processor, 64GB of RAM, and an NVIDIA RTX 4090 GPU, ensuring real-time inference and planning.
\vspace{-15pt}
\begin{figure}[h]
    \centering
    \includegraphics[width=\linewidth]{Figures/supp/hardware_setup.pdf}
    \caption{Hardware Configuration.}
    \label{fig:supp_hardware}
    \vspace{-10pt}
\end{figure}
\vspace{-10pt}
%%%%%%%%%%%%%%%%%%%%%%%%%%%%%%%%%%%%%%%%%%%%%%%%%%%%%%%%%%%%%%%%%%%%%%%%%%%%%%%
\subsection{Prompt for Querying VLM}
\label{sec:prompt}
This paper uses GPT-4O from the OpenAI API as VLM. Below, we provide specific prompts and corresponding JSON schema to enable VLM to deliver structured outputs.

\noindent\textbf{Task-relevant object grounding and stage partitioning.}
Takes task instructions and the object detection results from the VFM as inputs. Generates the task-relevant object IDs and the stage partitioning results (Section \textcolor{cvprblue}{3.1} of the main manuscript). The prompt is available for download \href{https://raw.githubusercontent.com/omnimanip/omnimanip.github.io/refs/heads/save/prompts/task_stage_partition.json}{\textcolor{my_pink}{here}}.

\noindent\textbf{Grounding Interaction Point.}
Takes task instructions and object images processed by the SCAFFOLD visual prompting mechanism as inputs. Generates the IDs of task-relevant interaction points on the object (Section \textcolor{cvprblue}{3.2} of the main manuscript). The prompt is available for download \href{https://raw.githubusercontent.com/omnimanip/omnimanip.github.io/refs/heads/save/prompts/interaction_point_generation.json}{\textcolor{my_pink}{here}}.

\noindent\textbf{Captioning Interaction Direction.}
Takes object images with candidate interaction directions and descriptions of task-relevant object parts as inputs. Generates textual descriptions of the functionality associated with each candidate interaction direction (Section \textcolor{cvprblue}{3.2} of the main manuscript). The prompt is available for download \href{https://raw.githubusercontent.com/omnimanip/omnimanip.github.io/refs/heads/save/prompts/interaction_direction_generation_part_1.json}{\textcolor{my_pink}{here}}.

\noindent\textbf{Determining Interaction Direction.}
Takes task instructions and textual descriptions of the functionality associated with candidate directions as inputs. Generates a ranking of the candidates according to the relevance between the directions and task instructions (Section \textcolor{cvprblue}{3.2} of the main manuscript). The prompt is available for download \href{https://raw.githubusercontent.com/omnimanip/omnimanip.github.io/refs/heads/save/prompts/interaction_direction_generation_part_2.json}{\textcolor{my_pink}{here}}.

\noindent\textbf{Self-correction via RRC.}
Takes rendered images of the interaction results as inputs.
Determines whether the interaction can be successful or if refinement is needed(Section \textcolor{cvprblue}{3.3} of the main manuscript). The prompt is available for download \href{https://raw.githubusercontent.com/omnimanip/omnimanip.github.io/refs/heads/save/prompts/RRC.json}{\textcolor{my_pink}{here}}.

%%%%%%%%%%%%%%%%%%%%%%%%%%%%%%%%%%%%%%%%%%%%%%%%%%%%%%%%%%%%%%%%%%%%%%%%%%%%%%%
\subsection{Implementation Details of Method}
\noindent\textbf{Object Canonicalization.}
In this paper, we employs the single-view object generation model TripoSR to generate 3D object meshes $\mathcal{M}$ from single-view RGB images. However, such reconstructions inherently face ambiguities in scale, rotation, and translation. To resolve these ambiguities, we estimate the similarity transformation $\{s, \mathbf{R}, \mathbf{t}\}$ between the reconstructed mesh and the canonical object space using the observed point cloud $\mathcal{P}_{\text{obs}}$.
First, the 6D object pose is estimated using Omni6DPose, and $\mathcal{P}_{\text{obs}}$ is transformed into the canonical point cloud $\mathcal{P}_{\text{can}}$. With known correspondences between $\mathcal{P}_{\text{can}}$ and the reconstructed mesh $\mathcal{M}$, the Umeyama~\cite{umeyama} algorithm is applied to compute the similarity transformation. This transformation includes the scale factor $s \in \mathbb{R}^+$, the rotation matrix $\mathbf{R} \in \text{SO}(3)$, and the translation vector $\mathbf{t} \in \mathbb{R}^3$.

\noindent\textbf{Functional Grasping.} 
We apply special processing to the `grasp' stage by directly generating primitives using universal grasp models \cite{anygrasp, gsnet}, without using RRC. Multiple grasp points on an object that meet the task requirements are obtained through \cite{scaffold}. For each point, a Gaussian distribution is generated and then superimposed, resulting in a continuous heatmap. This heatmap is used to post-process and filter the multiple grasp poses predicted by the grasp model, ultimately identifying the most suitable grasp pose.

\noindent\textbf{Rendering Details of RRC.} 
After obtaining the canonicalized object mesh and deriving the interaction vector and corresponding target pose as described in Section \ref{sec:primitives}, we set the pose for all meshes and render them using Pyrender. Before rendering, we apply the method from \cite{inpainting} to inpaint the original areas of the rendered object in the image, preventing interference with the VLM.

\noindent\textbf{Action Primitives based on Constraints.} We define the following atomic actions for VLM to select and complete constraint-based manipulation. (a) Grasp: Move to 8cm in front of the grasp pose, move forward and close the gripper. (b) Place: move to $v$cm in front of the target pose, move to the target pose and open the gripper. (c) Push: move to $v$cm in front of the target pose, close the gripper, and move to the target pose. (d) Pull: move to $v$cm in behind of the target pose (e) Rotate: rotate $v$ degrees along the interaction vector. (f) Pour: move to the target point and then rotate around that point to achieve the desired orientation.  $v$ is the distance predicted by VLM.

%%%%%%%%%%%%%%%%%%%%%%%%%%%%%%%%%%%%%%%%%%%%%%%%%%%%%%%%%%%%%%%%%%%%%%%%%%%%%%%

%%%%%%%%%%%%%%%%%%%%%%%%%%%%%%%%%%%%%%%%%%%%%%%%%%%%%%%%%%%%%%%%%%%%%%%%%%%%%%%
\subsection{System Error Breakdown}
\label{sec:supp_error_breakdown}
In this section, we conduct an empirical study by manually examining the failure cases of experiments in Table \ref{table:main_table}, calculating the likelihood of each module causing failures in the pipeline. The results are shown in Figure \ref{fig:supp_error_breakdown}. Among the different modules, object canonicalization (3D AIGC and Pose estimation) is relatively prone to failure. Our qualitative analysis indicates that the main reason is the significant decline in the quality stability of \cite{triposr} generation when small objects are positioned far from the camera. Therefore, it is recommended to use high-resolution cameras and capture images as close to the objects as possible. Additionally, the Grasping module and the VFM-based object grounding module also contribute to some errors. In contrast, the module that extracts interaction points and directions based on VLM is more stable, contributing less to failures. Lastly, factors such as unsolvable inverse kinematics (IK) for the robotic arm and collisions during execution also lead to some failure cases.
\begin{figure}[h]
    \centering
    \includegraphics[width=\linewidth]{Figures/supp/Error_Breakdown.pdf}
    \vspace{-20pt}
    \caption{
    System error breakdown.
    }
    \label{fig:supp_error_breakdown}
    \vspace{-20pt}
\end{figure}

%%%%%%%%%%%%%%%%%%%%%%%%%%%%%%%%%%%%%%%%%%%%%%%%%%%%%%%%%%%%%%%%%%%%%%%%%%%%%%%
\subsection{Imitation Learning Results Across Tasks} 
\label{sec:supp_il}
% \Tref{table:supp_il_policy}
% \Fref{fig:supp_il_trajectory}

\begin{table}[h]
    \centering
    \input{Tables/supp_il_policy.tex}
    \caption{
    Behavior cloning with demonstrations from OmniManip.
    }
    \label{table:supp_il_policy}
\end{table}

We deployed OmniManip in Isaac Sim for autonomous demonstrations collection. ~\Fref{fig:supp_il_trajectory} illustrates the overall trajectory distribution for the tasks 'insert flower' and 'fit lid onto teapot', showcasing a notable diversity in the data. As shown in~\Tref{table:supp_il_policy}, the policy \cite{diffusion_policy} trained using demonstration trajectories generated by OmniManip achieved an average accuracy of 86.93\% across five tasks, which partially validates the quality of the demonstrations generated by OmniManip.
\begin{figure}[h]
    \centering
    \includegraphics[width=\linewidth]{Figures/supp/sim.pdf}
    \caption{Trajectories visualization from OmniManip.}
    \label{fig:supp_il_trajectory}
    \vspace{-15pt}
\end{figure}

%%%%%%%%%%%%%%%%%%%%%%%%%%%%%%%%%%%%%%%%%%%%%%%%%%%%%%%%%%%%%%%%%%%%%%%%%%%%%%%
\subsection{Comprehensive Limitation Analysis}
\label{sec:supp_limitation}

\noindent\textbf{Stability and Trade-offs in 3D-AIGC.}
OmniManip's closed-loop planning reduces sensitivity to various components, but 3D AIGC model quality remains crucial. Balancing stability and efficiency is key. To ensure fast inference in real-world tests, we used \cite{triposr} to generate a 3D mesh in under half a second. This efficient option can yield poor meshes with low resolution or unusual angles. For better results, users can choose higher-quality models like \cite{One2345++}, though this increases computational time significantly.

\noindent\textbf{Challenges in General Pose Estimation.} General pose estimation \cite{omni6dpose} shows instability with certain rare objects, such as uncommon categories and transparent items. The estimated 6D pose at this point may not correctly align with the object's functional axis, reducing the sampling efficiency of OmniManip. However, the presence of RRC allows OmniManip to compensate to some extent.

\noindent\textbf{Heavy VLM Calls.} Multiple VLM calls average a cost of 11,000 tokens per plan, which represents a large computational overhead. However, most modules within the system can be executed and optimized in parallel to significantly enhance efficiency.

\noindent\textbf{Complex Task Handling with OmniManip.} It is challenging for OmniManip to handle complex tasks that are difficult to represent structurally, such as manipulating deformable objects. However, we believe that OmniManip, with its dual closed-loop features, continues to advance in the field of general object manipulation.

\begin{figure*}[t]
    \centering
    \includegraphics[width=\linewidth]{Figures/supp/all_pipeline_visualization/close_laptop.pdf}
    \vspace{-15pt}
    \caption{Result of task `Close lid of laptop'.}
    \vspace{-15pt}    \label{fig:supp_close_laptop}
\end{figure*}

%%%%%%%%%%%%%%%%%%%%%%%%%%%%%%%%%%%%%%%%%%%%%%%%%%%%%%%%%%%%%%%%%%%%%%%%%%%%%%%
\subsection{Inference Results Example}
\label{sec:supp_qualitative}
% \noindent\textbf{Qualitative Visualization.}
To provide a more detailed explanation of our approach, this section includes qualitative visualizations of three real-world tasks. These visualizations illustrate the key steps at each stage, such as identifying interaction points, providing textual descriptions of interaction directions and their corresponding task-related sequences, and showcasing the results of the self-correction phase. Each stage of our method is clearly and intuitively depicted. The tasks are: (a) Close lid of laptop (Figure \ref{fig:supp_close_laptop}) (b) Insert pen into holder (Figure \ref{fig:supp_insert_pen}) and (c) Pick up cup onto dish (Figure \ref{fig:supp_pick_cup}).

\begin{figure*}[t]
    \centering
    \includegraphics[width=0.95\linewidth]{Figures/supp/all_pipeline_visualization/insert_pen.pdf}
    \caption{Result of task `Insert pen into holder'.}
    \label{fig:supp_insert_pen}
\end{figure*}

\begin{figure*}[t]
    \centering
    \includegraphics[width=0.95\linewidth]{Figures/supp/all_pipeline_visualization/pick_cup_onto_dish.pdf}
    \caption{Result of task `Pick up cup onto dish'.}
    \label{fig:supp_pick_cup}
\end{figure*}
